# Supplementary material for: Centennial-scale variability of the Atlantic Meridional Circulation in CMIP6 models shaped by Arctic-North Atlantic interactions and sea ice biases
Source: arXiv:2406.09919 ancillary file (2024-06-14)
Supplement: Supplementary file 1 [file Supplement.pdf]

# Supporting Information for "Centennial-scale variability of the Atlantic Meridional Circulation in CMIP6 models shaped by Arctic–North Atlantic interactions and sea ice biases"

Oliver Mehling[1], Katinka Bellomo[1,2], and Jost von Hardenberg[1,2]

[1]Department of Environment, Land and Infrastructure Engineering, Politecnico di Torino, Turin, Italy

[2]National Research Council of Italy, Institute of Atmospheric Sciences and Climate (CNR-ISAC), Turin, Italy

## Contents of this file

1. Table S1

2. Figures S1 to S9

## References

Boucher, O., Denvil, S., Levavasseur, G., Cozic, A., Caubel, A., Foujols, M.-A., ... Cheruy, F. (2018). *IPSL IPSL-CM6A-LR model output prepared for CMIP6 CMIP piControl. Version 20200326.* Earth System Grid Federation. doi: 10.22033/ESGF/CMIP6.5251

Boucher, O., Servonnat, J., Albright, A. L., Aumont, O., Balkanski, Y., Bastrikov, V., ... Vuichard, N. (2020). Presentation and Evaluation of the IPSL-CM6A-LR Climate Model. *J. Adv. Model. Earth Syst.*, *12*, e2019MS002010. doi: 10.1029/2019MS002010

Danabasoglu, G., Lamarque, J.-F., Bacmeister, J., Bailey, D. A., DuVivier, A. K., Edwards, J., ... Strand, W. G. (2020). The Community Earth System Model Version 2 (CESM2). *J. Adv. Model. Earth Syst.*, *12*, e2019MS001916. doi: 10.1029/2019MS001916

Danabasoglu, G., Lawrence, D., Lindsay, K., Lipscomb, W., & Strand, G. (2019). *NCAR CESM2 model output prepared for CMIP6 CMIP piControl. Version 20190917.* Earth System Grid Federation. doi: 10.22033/ESGF/CMIP6.7733

Döscher, R., Acosta, M., Alessandri, A., Anthoni, P., Arsouze, T., Bergman, T., ... Zhang, Q. (2022). The EC-Earth3 Earth system model for the Coupled Model Intercomparison Project 6. *Geosci. Model Dev.*, *15*, 2973–3020. doi: 10.5194/gmd-15-2973-2022

EC-Earth Consortium. (2019). *EC-Earth-Consortium EC-Earth3 model output prepared for CMIP6 CMIP piControl. Version 20210601.* Earth System Grid Federation. doi:

10.22033/ESGF/CMIP6.4842

Kuhlbrodt, T., Jones, C. G., Sellar, A., Storkey, D., Blockley, E., Stringer, M., ... Walton, J. (2018). The Low-Resolution Version of HadGEM3 GC3.1: Development and Evaluation for Global Climate. *J. Adv. Model. Earth Syst.*, *10*, 2865–2888. doi: 10.1029/2018MS001370

Mauritsen, T., Bader, J., Becker, T., Behrens, J., Bittner, M., Brokopf, R., ... Roeckner, E. (2019). Developments in the MPI-M Earth System Model version 1.2 (MPI-ESM1.2) and Its Response to Increasing CO2. *J. Adv. Model. Earth Syst.*, *11*, 998–1038. doi: 10.1029/2018MS001400

Neubauer, D., Ferrachat, S., Siegenthaler-Le Drian, C., Stoll, J., Folini, D. S., Tegen, I., ... Lohmann, U. (2019). *HAMMOZ-Consortium MPI-ESM1.2-HAM model output prepared for CMIP6 CMIP piControl. Version 20200120.* Earth System Grid Federation. doi: 10.22033/ESGF/CMIP6.5037

Ridley, J., Menary, M., Kuhlbrodt, T., Andrews, M., & Andrews, T. (2018). *MOHC HadGEM3-GC31-LL model output prepared for CMIP6 CMIP piControl. Version 20211103.* Earth System Grid Federation. doi: 10.22033/ESGF/CMIP6.6294

Sellar, A. A., Jones, C. G., Mulcahy, J. P., Tang, Y., Yool, A., Wiltshire, A., ... Zerroukat, M. (2019). UKESM1: Description and Evaluation of the U.K. Earth System Model. *J. Adv. Model. Earth Syst.*, *11*, 4513–4558. doi: 10.1029/2019MS001739

Swart, N. C., Cole, J. N., Kharin, V. V., Lazare, M., Scinocca, J. F., Gillett, N. P., ... Sigmond, M. (2019b). *CCCma CanESM5 model output prepared for CMIP6 CMIP piControl. Version 20190429.* Earth System Grid Federation. doi: 10.22033/ESGF/

CMIP6.3673

Swart, N. C., Cole, J. N. S., Kharin, V. V., Lazare, M., Scinocca, J. F., Gillett, N. P., … Winter, B. (2019a). The Canadian Earth System Model version 5 (CanESM5.0.3). *Geosci. Model Dev.*, *12*, 4823–4873. doi: 10.5194/gmd-12-4823-2019

Tang, Y., Rumbold, S., Ellis, R., Kelley, D., Mulcahy, J., Sellar, A., … Jones, C. (2019). *MOHC UKESM1.0-LL model output prepared for CMIP6 CMIP piControl. Version 20200828.* Earth System Grid Federation. doi: 10.22033/ESGF/CMIP6.6298

Tegen, I., Neubauer, D., Ferrachat, S., Siegenthaler-Le Drian, C., Bey, I., Schutgens, N., … Lohmann, U. (2019). The global aerosol–climate model ECHAM6.3–HAM2.3 – Part 1: Aerosol evaluation. *Geosci. Model Dev.*, *12*, 1643–1677. doi: 10.5194/gmd-12-1643-2019

Wieners, K.-H., Giorgetta, M., Jungclaus, J., Reick, C., Esch, M., Bittner, M., … Roeckner, E. (2019). *MPI-M MPI-ESM1.2-LR model output prepared for CMIP6 CMIP piControl. Version 20190710.* Earth System Grid Federation. doi: 10.22033/ESGF/CMIP6.6675

Ziehn, T., Chamberlain, M., Lenton, A., Law, R., Bodman, R., Dix, M., … Druken, K. (2019). *CSIRO ACCESS-ESM1.5 model output prepared for CMIP6 CMIP piControl. Version 20210316.* Earth System Grid Federation. doi: 10.22033/ESGF/CMIP6.4312

Ziehn, T., Chamberlain, M. A., Law, R. M., Lenton, A., Bodman, R. W., Dix, M., … Srbinovsky, J. (2020). The Australian Earth System Model: ACCESS-ESM1.5. *J. South. Hemisphere Earth Syst. Sci.*, *70*, 193–214. doi: 10.1071/ES19035

**Table S1.** CMIP6 models and simulations used in this study

| Model (Institution) | Ocean Component | Ensemble member | Years | $S_{\mathrm{ref}}$ | Model citation | Simulation reference |
|---|---|---|---|---|---|---|
| **ACCESS-ESM1-5** (CSIRO) | MOM5.1 | r1i1p1f1 | 1000 | 34.73 | Ziehn et al. (2020) | Ziehn et al. (2019) |
| **CanESM5** (CCCma) | NEMO3.4+ | r1i1p2f1 | 1051 | 34.27 | Swart et al. (2019a) | Swart et al. (2019b) |
| **CESM2** (NCAR) | POP2 | r1i1p1f1 | 1200 | 34.69 | Danabasoglu et al. (2020) | Danabasoglu et al. (2019) |
| **EC-Earth3** (EC-Earth Consortium) | NEMO3.6 | r2i1p1f1 | 1255 | 34.59 | Döscher et al. (2022) | EC-Earth Consortium (2019) |
| **HadGEM3-GC31-LL** (MOHC) | NEMO3.6 | r1i1p1f1 | 2000 | 34.54 | Kuhlbrodt et al. (2018) | Ridley et al. (2018) |
| **IPSL-CM6A-LR** (IPSL) | NEMO3.6 | r1i1p1f1 | 2000 | 34.59 | Boucher et al. (2020) | Boucher et al. (2018) |
| **MPI-ESM-1-2-HAM** (HAMMOZ Consortium) | MPIOM1.63 | r1i1p1f1 | 1000 | 34.65 | Tegen et al. (2019) | Neubauer et al. (2019) |
| **MPI-ESM1-2-LR** (MPI-M) | MPIOM1.63 | r1i1p1f1 | 1000 | 34.66 | Mauritsen et al. (2019) | Wieners et al. (2019) |
| **UKESM1-0-LL** (MOHC) | NEMO3.6 | r1i1p1f2 | 1880[a] | 34.52 | Sellar et al. (2019) | Tang et al. (2019) |

[a] First 1100 years only for so, vo, uo

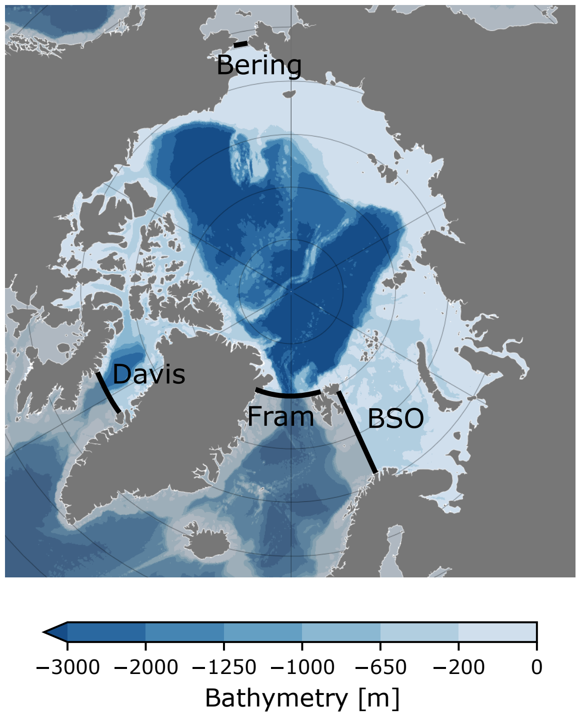


**Figure S1.** Map of the Arctic Ocean domain and straits

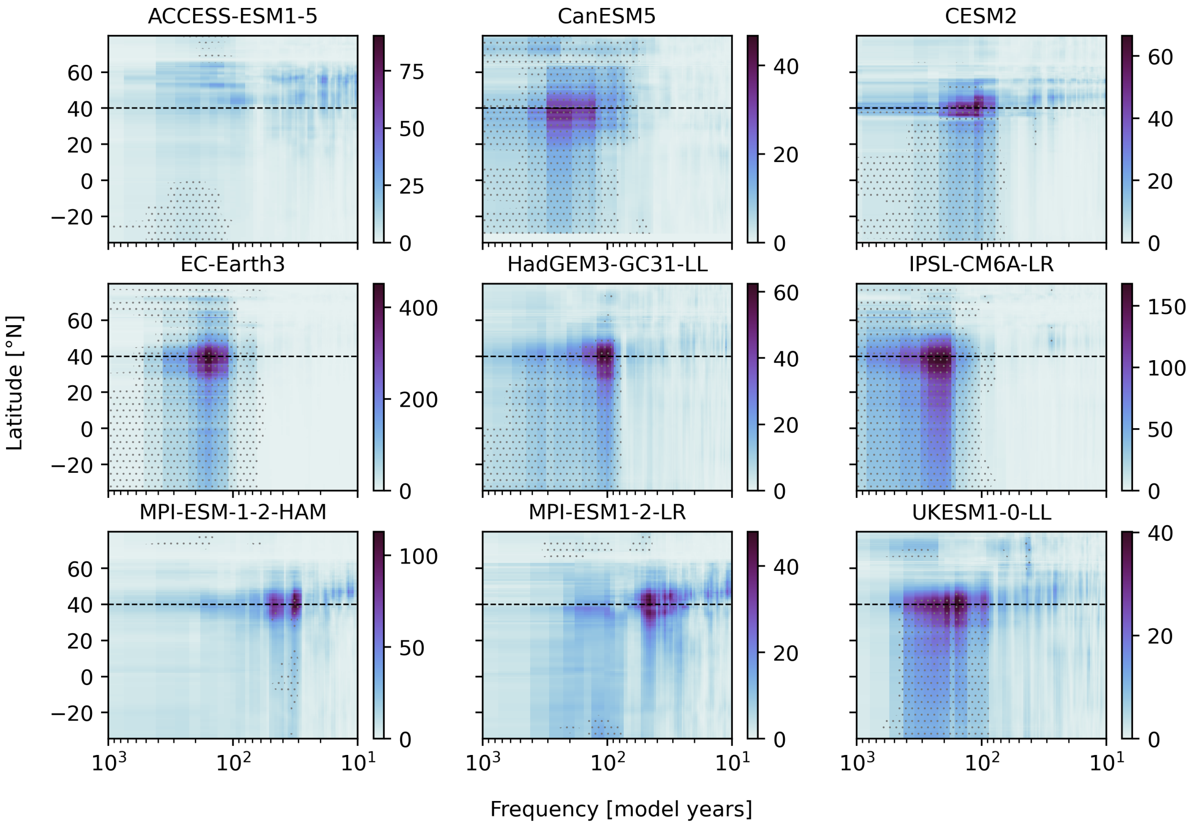


**Figure S2.** AMOC power spectrum by latitude for each model. Power that exceeds the 99% significance threshold is indicated by stippling.

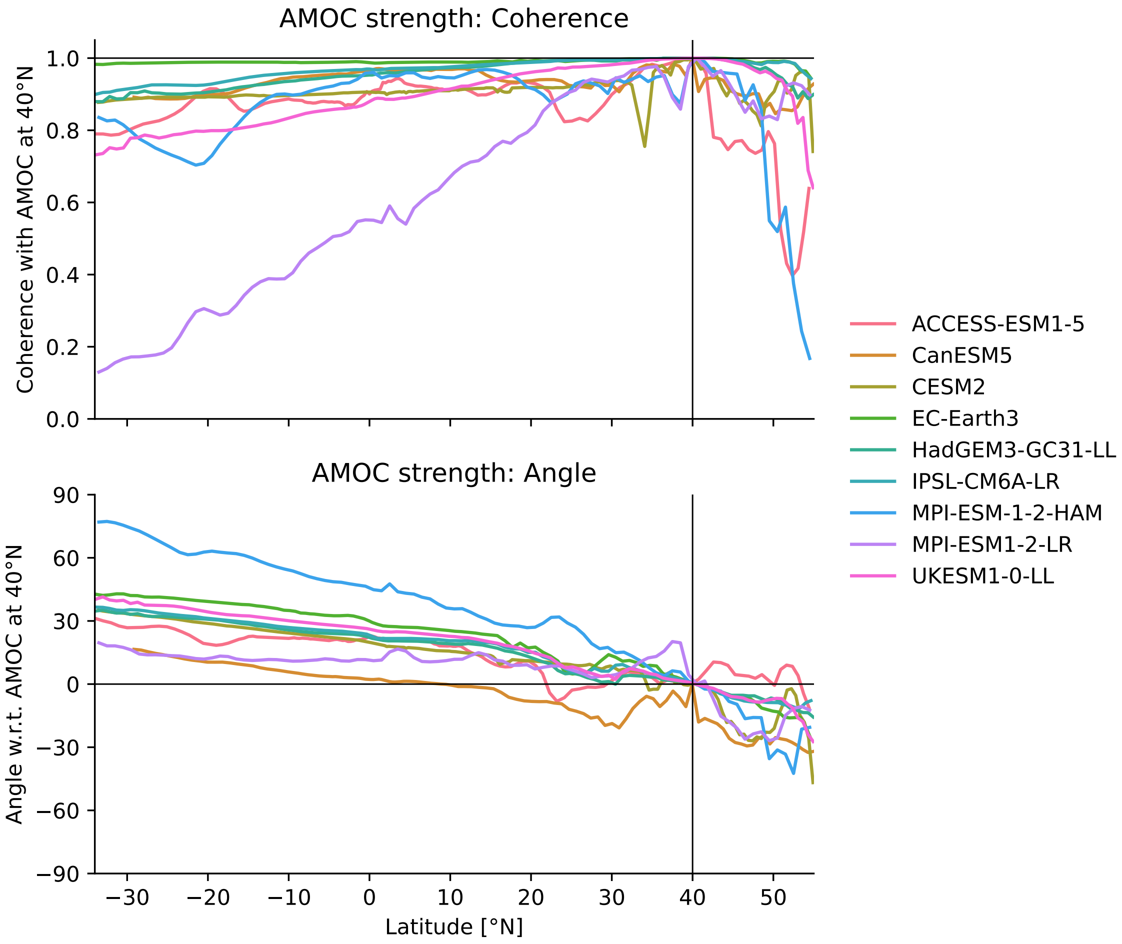


**Figure S3.** Multi-taper coherence and angle between the AMOC strength by latitude and the AMOC at 40°N. Cross-spectra were averaged over the period range 100–250 years before computing magnitude and angle.

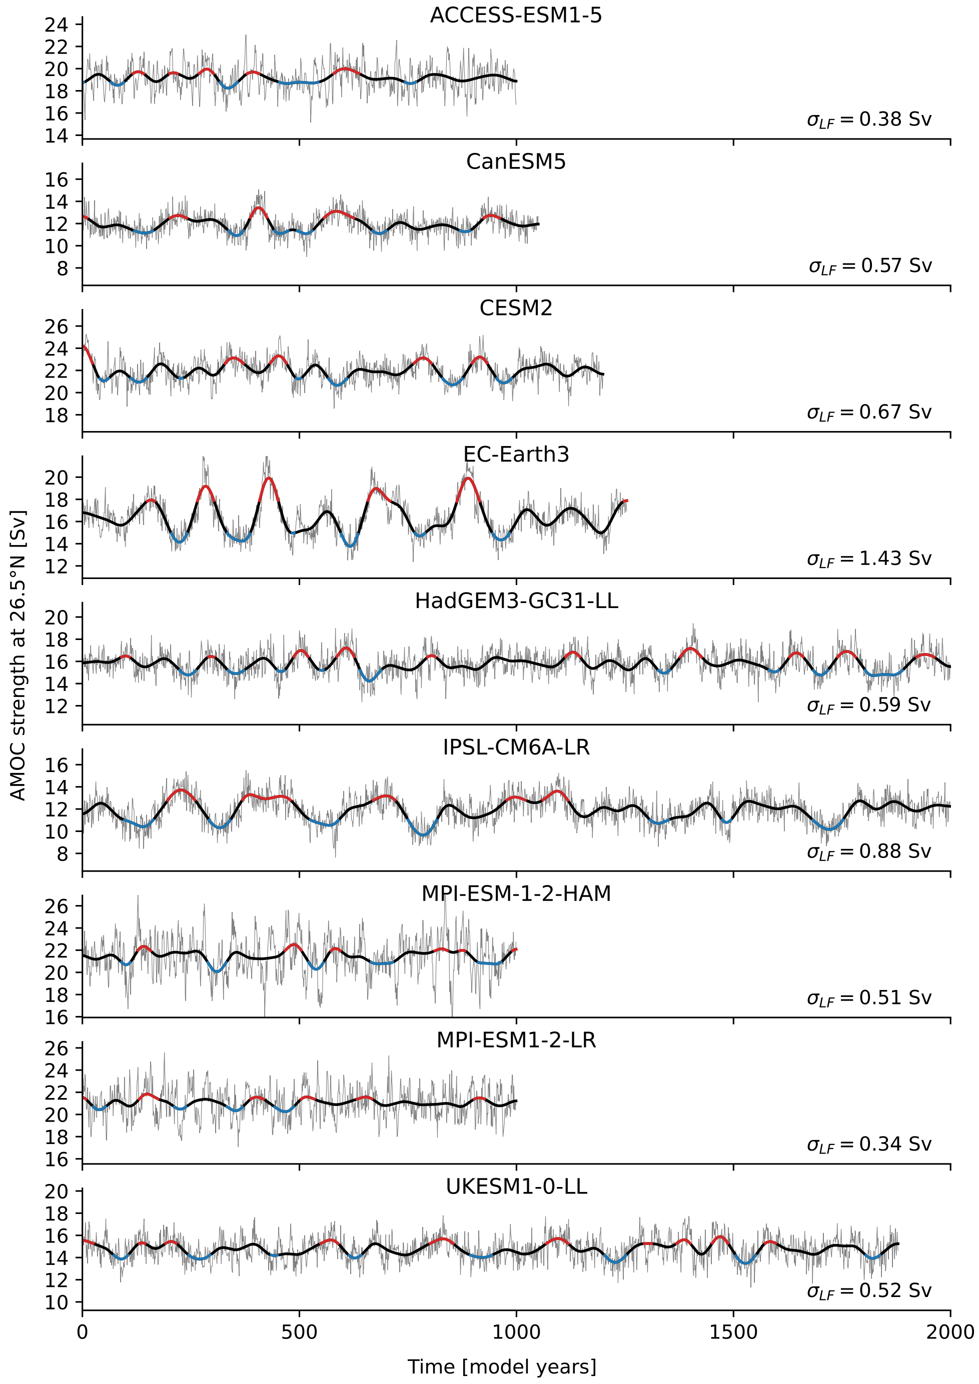


**Figure S4.** Detrended annual mean and 70-year low-pass filtered AMOC time series at 40°N. Intervals used for the calculation of "strong AMOC" and "weak AMOC" composites are highlighted in red and blue, respectively. The low-pass filtered standard deviation of AMOC strength is given in the bottom right for each model. (Note that y-axes cover +/− 5 Sv around the mean AMOC strength, which differs between models.)

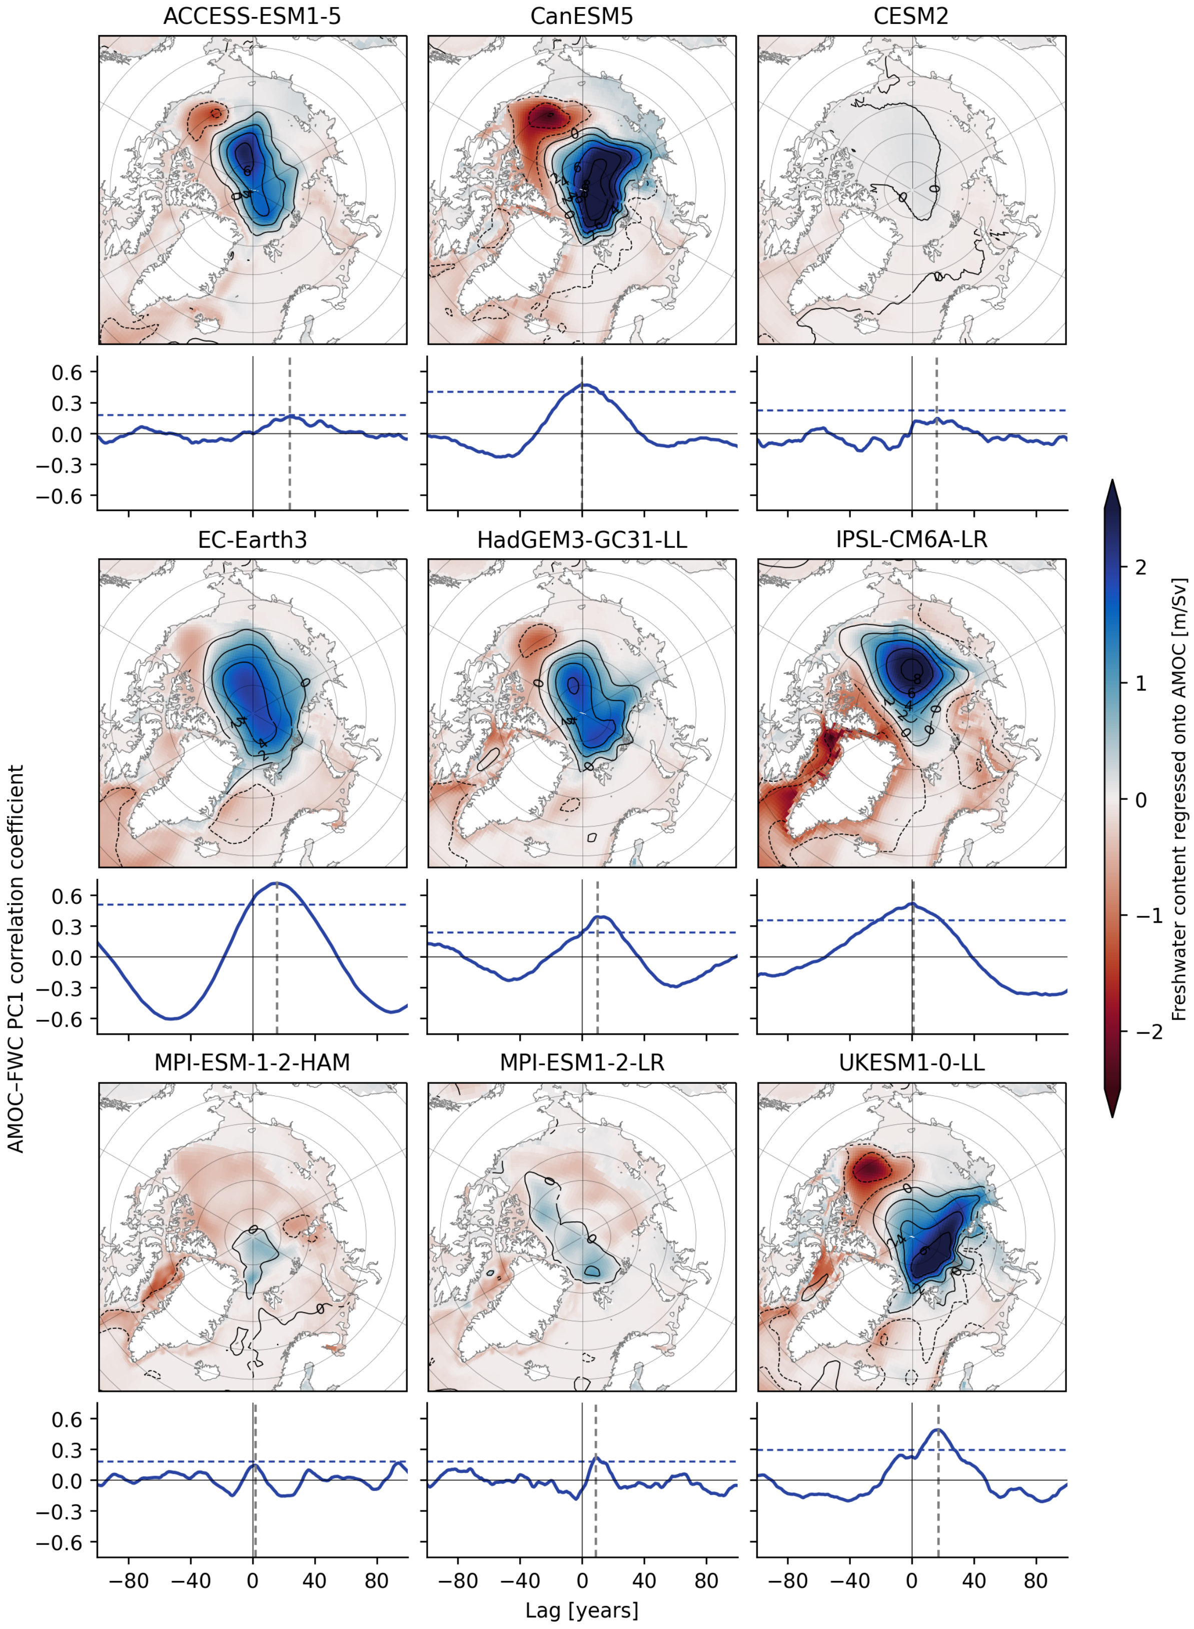


**Figure S5.** Same as Fig. 2, but regression patterns are taken at the lag where the

June 14, 2024, 10:48am

AMOC–PC1 correlation is at its maximum (grey dashed vertical lines in the line plots).

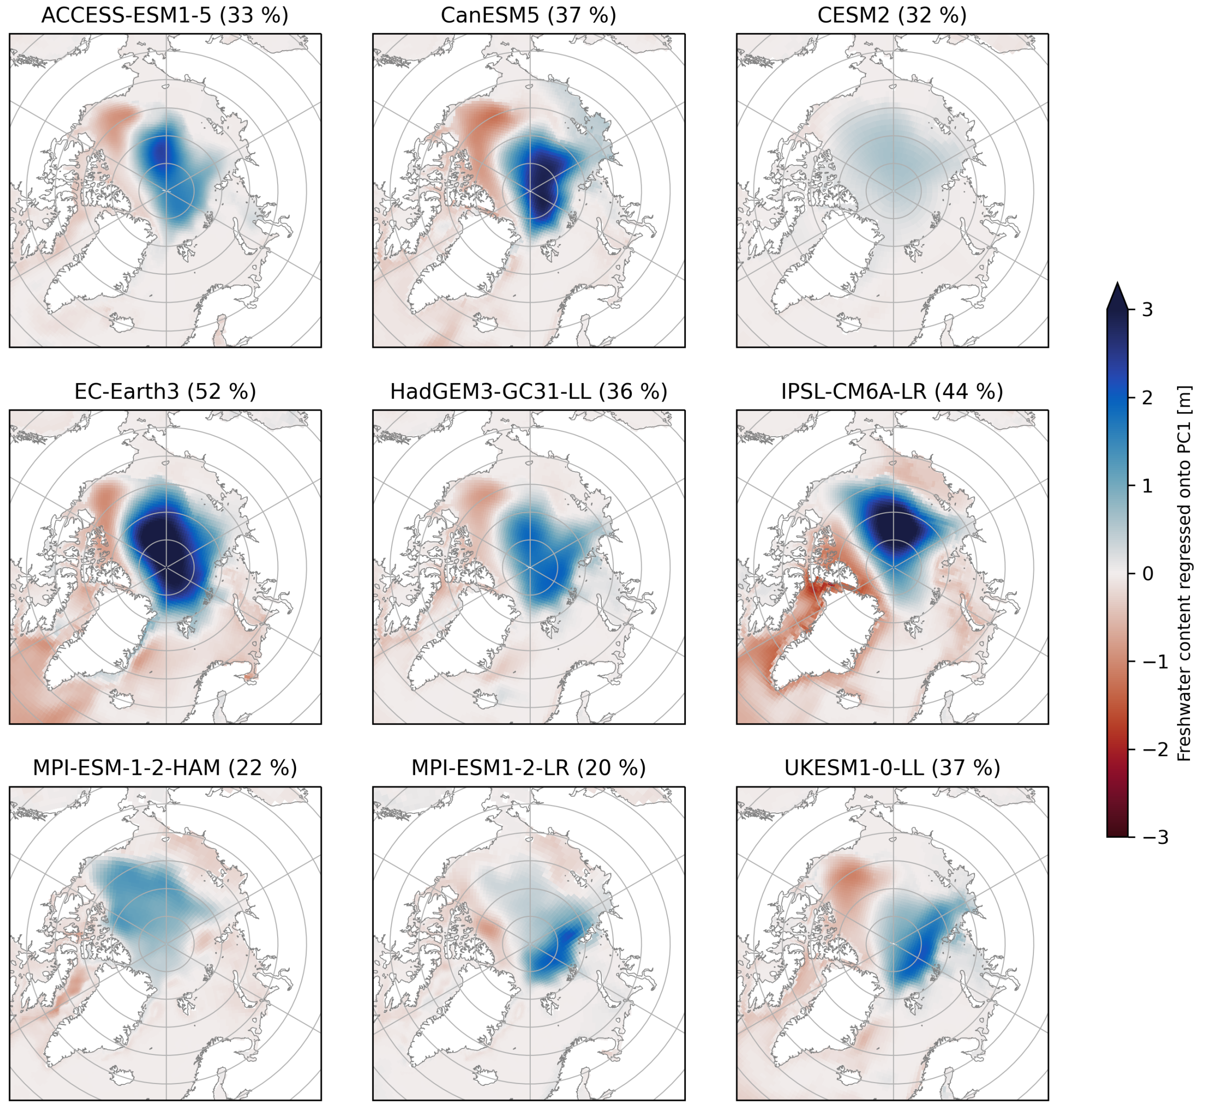


**Figure S6.** First EOF of annual mean Arctic Ocean freshwater content, obtained by regressing the (standardized) PC1 onto the freshwater content fields. Subtitles indicate the percentage of variance explained.

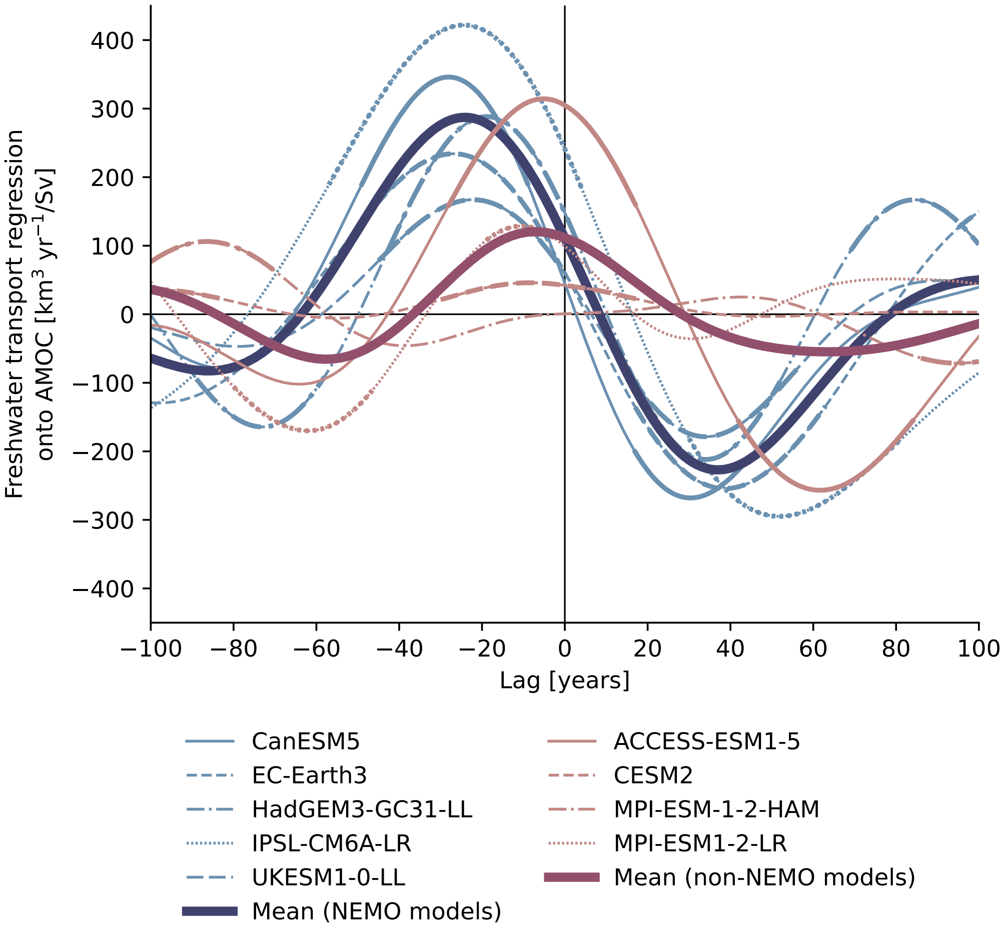


**Figure S7.** Low-pass filtered freshwater transport across Fram Strait regressed onto AMOC strength. Significant lagged regression coefficients are indicated by thicker lines and calculated as in Fig. 2. Blue lines: NEMO models, red lines: non-NEMO models. Multi-model means for the two groups are shown with darker, solid lines.

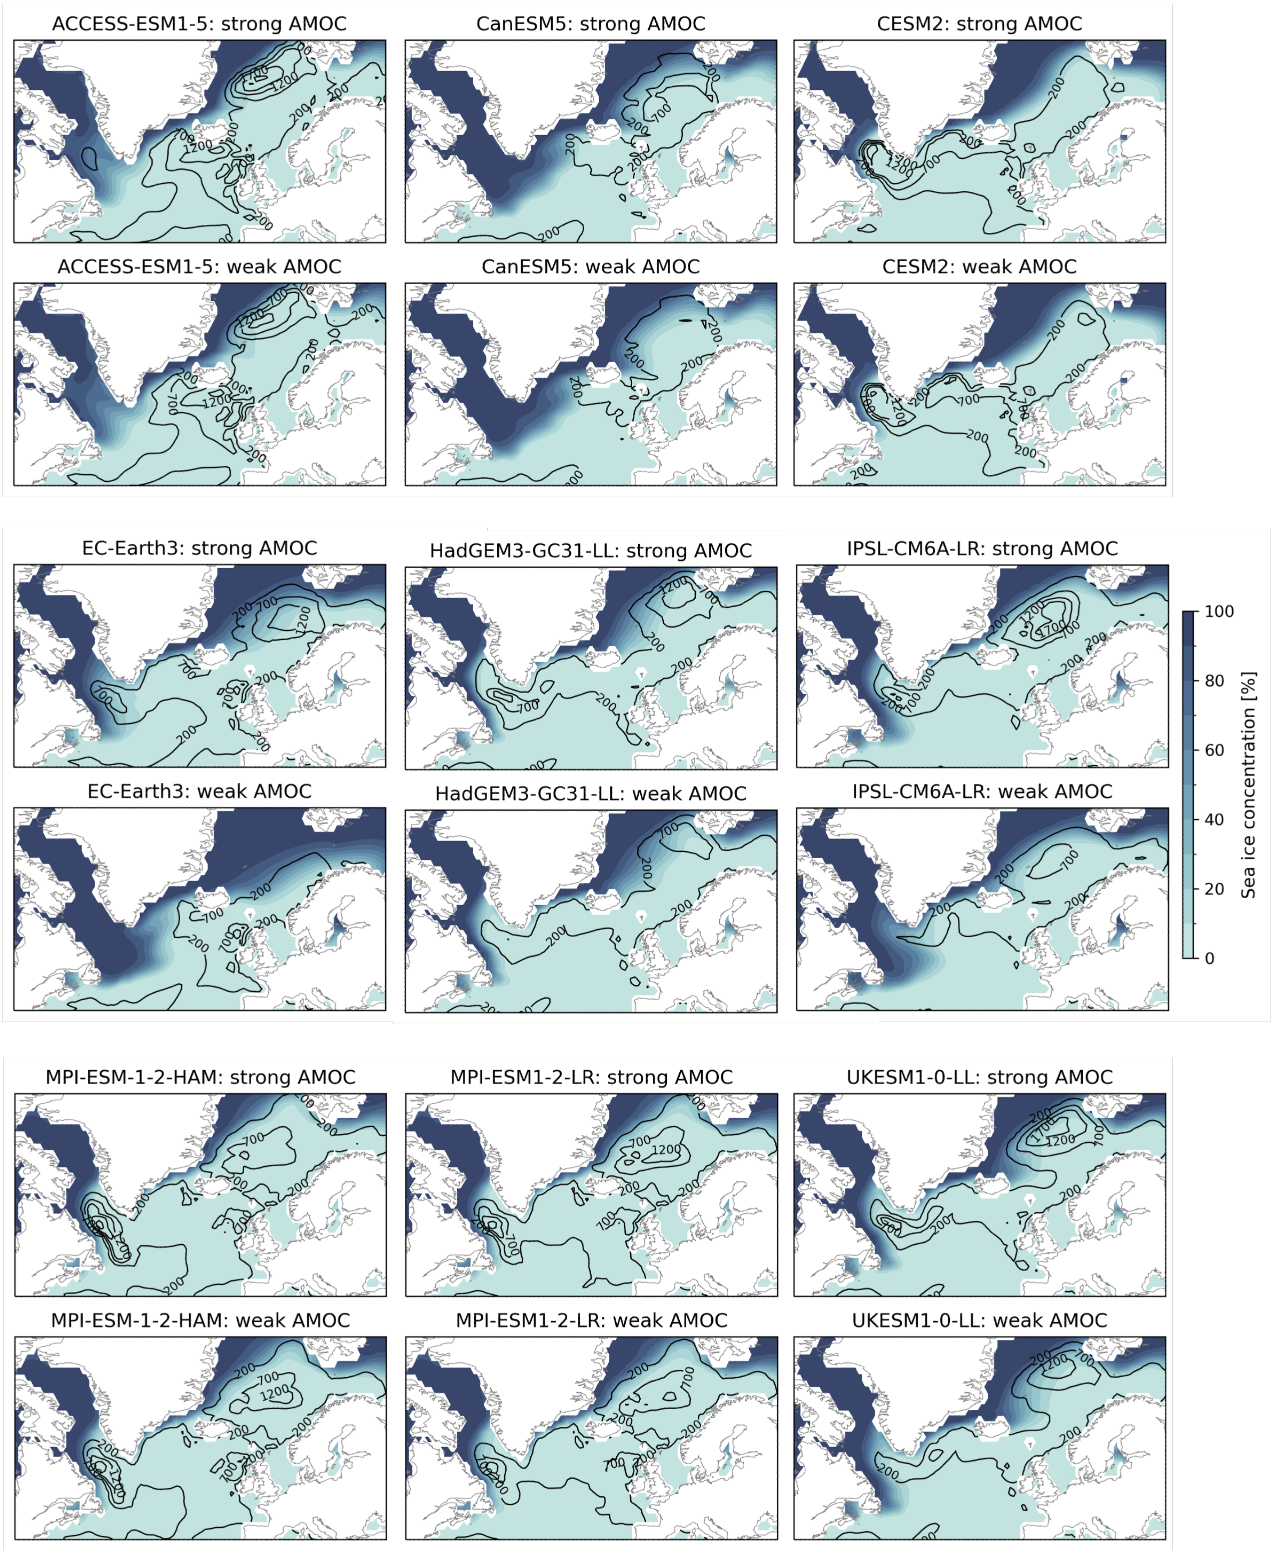


**Figure S8.** Same as Fig. 3a-d, but for all nine models.

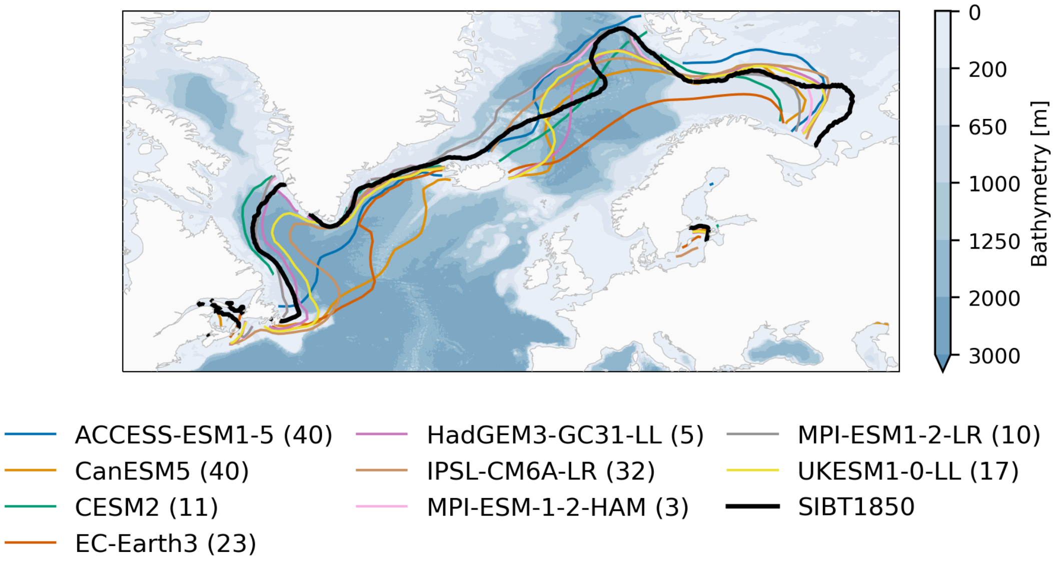


**Figure S9.** Same as Fig. 3e, but for ensemble means of the CMIP6 historical simulations (1850–2014) and SIBT1850 averaged over the same period. The number of ensemble members is given in brackets for each model.
